# Supplementary material for: Sisyphus Thermalization of Photons in a Cavity-Coupled Double Quantum Dot
Source: arXiv:1512.01248 source file (2016-10-11)
Supplement: Supplementary file 1 [file LZS_PRL_Supp_v2.pdf]

# Supplemental material to the manuscript: "Sisyphus Thermalization of Photons in a Cavity-Coupled Double Quantum Dot"

M. J. Gullans,[1,2] J. Stehlik,[3] Y.-Y. Liu,[3] C. Eichler,[3] J. R. Petta,[3] and J. M. Taylor[1,2]

[1] *Joint Quantum Institute, National Institute of Standards and Technology, Gaithersburg, Maryland 20899, USA*

[2] *Joint Center for Quantum Information and Computer Science, University of Maryland, College Park, Maryland 20742, USA*

[3] *Department of Physics, Princeton University, Princeton, New Jersey 08544, USA*

## PHOTON CORRELATION FUNCTIONS

The master equation for the DQD with $g_c = 0$ [Eq. (10) in the main text] can be used to evaluate all correlation functions of the form $\langle \prod_{i=1}^{n} \sigma_{\nu_i}(t_i)\rangle$ using the quantum regression theorem [S1]. In particular, the Louivillian associated with this master equation can be written as a matrix operating on the vector of the density matrix components $\rho_n = (\rho_n^{--}, \rho_n^{-+}, \rho_n^{+-}, \rho_n^{++})^T$ as

$$\mathcal{L} = \begin{pmatrix} -\gamma_+ & 0 & 0 & \gamma_- \\ 0 & -(\gamma - i\Delta) & 0 & 0 \\ 0 & 0 & -(\gamma + i\Delta) & 0 \\ \gamma_+ & 0 & 0 & -\gamma_- \end{pmatrix} \tag{S1}$$

where $\gamma = (\gamma_+ + \gamma_-)/2$ is the dephasing rate. The steady state is

$$\rho_{ss} = \left(\frac{\gamma_+}{2\gamma}, 0, 0, \frac{\gamma_-}{2\gamma}\right)^T \tag{S2}$$

A complete basis of operators acting on the two-level system is given by $\hat{\Lambda}_\pm = \sigma_\pm$ and $\hat{\Lambda}_z = \sigma_z - \langle\sigma_z\rangle$, which have the simple time evolution under $\mathcal{L}$

$$\left\langle \hat{\Lambda}_\pm(t)\right\rangle = \left\langle \hat{\Lambda}_\pm(0)\right\rangle e^{-(\gamma\pm i\Delta)t}, \tag{S3}$$

$$\left\langle \hat{\Lambda}_z(t)\right\rangle = \left\langle \hat{\Lambda}_z(0)\right\rangle e^{-2\gamma t}. \tag{S4}$$

We let $\tau$ be the permutation such that $t_{\tau(1)} > t_{\tau(2)} > ... > t_{\tau(n)}$, then Eq. (S3) and Eq. (S4) imply

$$\Big\langle \prod_i \hat{\Lambda}_{\nu_i}(t_i)\Big\rangle = f_{\nu_1,...,\nu_n}(t_1,...,t_n)\Big\langle \prod_i \hat{\Lambda}_{\nu_i}(0)\Big\rangle, \tag{S5}$$

$$f_{\nu_1,...,\nu_n}(t_1,...,t_n) = \prod_{i=1}^{n-1} e^{-\gamma_{\nu_{\tau(i)}}[t_{\tau(i)} - t_{\tau(i+1)}]}, \tag{S6}$$

where $\gamma_\pm = \gamma \pm i\Delta$ and $\gamma_z = 2\gamma$.

To find the correlation functions for the cavity field we treat the phonons as a Markovian bath and derive the Heisenberg-Langevin equations of motion for $a$ [S1]

$$\dot{a} = -\Big(\frac{\kappa + \hat{R}_a - \hat{R}_e}{2} + i\delta\Big)a + \sum_{m,\nu} \frac{2it_c g_c}{\hbar\omega_c} u_{yn_c}^{\nu m}\hat{\Lambda}_\nu \hat{F}_m \tag{S7}$$

$$+ \sum_m \frac{2it_c g_c}{\hbar\omega_c} u_{yn_c}^{zm}\langle\sigma_z\rangle \hat{F}_m + \sum_\nu \sigma_\nu(\hat{\mathcal{F}}_{a\nu} + \hat{\mathcal{F}}_{e\nu}^\dagger) + \hat{\mathcal{F}}_c,$$

$$\hat{R}_a = \sum_{n\ge 0} \gamma_{az}^n + \gamma_{a+}^n(1-\sigma_z)/2 + \gamma_{a-}^n(1+\sigma_z)/2, \tag{S8}$$

$$\hat{R}_e = \sum_{n\ge 0} \gamma_{ez}^n + \gamma_{e+}^n(1-\sigma_z)/2 + \gamma_{e-}^n(1+\sigma_z)/2. \tag{S9}$$

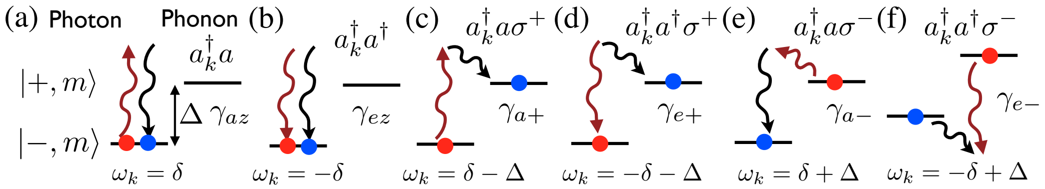


FIG. S1: Enumeration of phonon-assisted-photon processes starting from the state with the red circle and ending in the state with the blue circle. $|\pm, m\rangle$ are the Floquet states with quasi-energy $\pm\hbar\Delta$ and Floquet index $m$. All processes are drawn that *create* a phonon and either create or annihilate a photon. (a-b) Raman scattering process ending in the same state as the initial state with a phonon created at the frequency $\omega_k = \pm\delta = \pm(\omega_c - n_c\omega)$. (c-d) Processes starting in the lower Floquet state and ending in the upper state with a phonon created at frequency $\omega_k = \pm\delta - \Delta$. (e-f) Processes starting in the upper Floquet state and ending in the lower state with the creation of a photon at frequency $\omega_k = \pm\delta + \Delta$.

Each term in $\hat{R}_{e(a)}$ arises from the corresponding phonon-assisted, photon creation (annihilation) processes labeled in Fig. S1. They can be derived from Fermi's Golden rule for Floquet states as

$$\gamma_{az}^n = |u_{xn-n_c}^{z0}|^2 \mathcal{J}_R(\delta + n\omega), \tag{S10}$$

$$\gamma_{ez}^n = |u_{xn+n_c}^{z0}|^2 \mathcal{J}_R(-\delta + n\omega), \tag{S11}$$

$$\gamma_{a\pm}^n = |u_{xn-n_c}^{\pm m_{a\pm}}|^2 \mathcal{J}_R[\delta \pm \Delta + (n + m_{a\pm})\omega], \tag{S12}$$

$$\gamma_{e\pm}^n = |u_{xn+n_c}^{\pm m_{e\pm}}|^2 \mathcal{J}_R[-\delta \pm \Delta + (n + m_{e\pm})\omega], \tag{S13}$$

where $\mathcal{J}_R$ is defined in Eq. (12) of the main text, $m_{e\pm}$ is the closest integer to $(\delta \mp \Delta)/\omega$, and $m_{a\pm}$ is the closest integer to $(-\delta \mp \Delta)/\omega$. They each have an associated noise operator $\hat{\mathcal{F}}_{e(a)\nu}$ which satisfy

$$\left\langle \hat{\mathcal{F}}_{az}^\dagger(t)\hat{\mathcal{F}}_{az}(t')\right\rangle = \sum_{n\geq 0} \gamma_{az}^n n_p(\delta + n\omega)\delta(t - t'), \tag{S14}$$

$$[\hat{\mathcal{F}}_{az}(t), \hat{\mathcal{F}}_{az}^\dagger(t')] = \sum_{n\geq 0} \gamma_{az}^n \delta(t - t'), \tag{S15}$$

and similarly for the other noise operators. $\hat{\mathcal{F}}_c$ is the noise operator associated with the cavity decay $\kappa$ and satisfies

$$\left\langle \hat{\mathcal{F}}_c^\dagger(t)\hat{\mathcal{F}}_c(t')\right\rangle = \kappa\, n_p(\omega_c)\delta(t - t'), \tag{S16}$$

$$[\hat{\mathcal{F}}_c(t), \hat{\mathcal{F}}_c^\dagger(t')] = \kappa\, \delta(t - t') \tag{S17}$$

To calculate the correlation functions of $a$ we first approximate $\hat{R}_{e(a)}$ by their expectation values and formally integrate the equation for $a$

$$a(t) = a_c(t) + a_d(t) + a_f(t),$$

$$a_c(t) = \sum_m \frac{2it_c g_c}{\hbar\omega_c} \frac{u_{yn_c}^{zm}\langle\sigma_z\rangle \hat{F}_m(t)}{(\kappa + R_a - R_e)/2 + i(\delta + m\omega)} \tag{S18}$$

$$a_d(t) = \sum_{m,\nu} \frac{2it_c g_c}{\hbar\omega_c} u_{yn_c}^{\nu m} \hat{F}_m(t) \int_{-\infty}^t dt' e^{-[(\kappa + R_a - R_e)/2 + i\delta](t-t')} \hat{\Lambda}_\nu(t') e^{im\omega t'} \tag{S19}$$

$$a_f(t) = \int_{-\infty}^t dt' e^{-[(\kappa + R_a - R_e)/2 + i\delta](t-t')} \Big\{ \sum_\nu \sigma_\nu(t') \big[\hat{\mathcal{F}}_{a\nu}(t') + \hat{\mathcal{F}}_{e\nu}^\dagger(t')\big] + \hat{\mathcal{F}}_c(t') \Big\}. \tag{S20}$$

The resonator field has three distinct contributions: $a_c(t)$ describes coherent light arising from the strong driving of the DQD, $a_d(t)$ arises from the resonance fluorescence of the DQD and gives rise to anti-bunched light, and the $a_f(t)$ describes the thermal contributions to the light. $a_f$ has the

property that it only gives a non-zero expectation value when it is paired with $a_f^\dagger$, this allows for the simplification

$$\langle a^\dagger a\rangle = \langle a_f^\dagger a_f\rangle + \langle a_c^\dagger a_c\rangle + \langle a_d^\dagger a_d\rangle, \tag{S21}$$

$$g^{(2)}(0) = \frac{2\big[\langle a^\dagger a\rangle^2 - (\langle a_c^\dagger a_c\rangle - \langle a_d^\dagger a_d\rangle)^2\big] + \langle (a_c+a_d)^\dagger (a_c+a_d)^\dagger (a_c+a_d)(a_c+a_d)\rangle}{\langle a^\dagger a\rangle^2}, \tag{S22}$$

$$\approx \frac{2\big[\langle a^\dagger a\rangle^2 - (\langle a_c^\dagger a_c\rangle - \langle a_d^\dagger a_d\rangle)^2\big] + \langle a_d^\dagger a_d^\dagger a_d a_d\rangle}{\langle a^\dagger a\rangle^2}, \tag{S23}$$

where the we use the fact that $a_c$ is generally a small coherent field compared to $a_d$. From this formula, we see that antibunching will only occur when $\langle a_f^\dagger a_f\rangle \ll \langle a_d^\dagger a_d\rangle$ and $\langle a_d^\dagger a_d^\dagger a_d a_d\rangle \ll \langle a_d^\dagger a_d\rangle^2$. This second inequality always holds because of the strong phonon emission of the DQD. The large phonon decay rate implies that when the DQD emits a single photon it is unlikely that it will emit another photon the next time it is excited. This can be proved by looking at the scaling of the contributions of $a_d$ to the numerator of $g^{(2)}(0)$

$$\begin{aligned}
\langle a_d^\dagger a_d^\dagger a_d a_d\rangle &\sim \int_{-\infty}^{t} dt_1 \int_{-\infty}^{t_1} dt_2 \int_{-\infty}^{t_2} dt_3 \int_{-\infty}^{t_3} dt_4 \langle \hat\Lambda_z(t_1)\hat\Lambda_z(t_2)\hat\Lambda_z(t_3)\hat\Lambda_z(t_4)\rangle \\
&\times e^{-\frac{(\kappa+R_a-R_e)}{2}(4t-t_1-t_2-t_3-t_4)+i(\delta+m\omega)(t_1+t_2-t_3-t_4)} + \dots \\
&= \int_{-\infty}^{t} dt' \int_0^\infty d\tau_1 d\tau_2 d\tau_3\, e^{2(\kappa+R_a-R_e)(t-t')-\kappa(3\tau_1+2\tau_2+\tau_3)-i(\delta+m\omega)(\tau_1+2\tau_2+\tau_3)-2\gamma(\tau_1+\tau_2+\tau_3)} + \dots \\
&= \frac{1}{4(\kappa+R_a-R_e)(\gamma+i\delta)(2\gamma+i\delta)^2} + \dots .
\end{aligned} \tag{S24}$$

Due to Eq. (S5), all the additional terms take the same form and are of the same order of magnitude as Eq. (S24). These contributions should be compared to the typical size of the contribution to the denominator of $g^{(2)}(0)$

$$\begin{aligned}
\langle a_d^\dagger a_d\rangle &\sim \int_{-\infty}^{t} dt' \int_0^\infty d\tau e^{-(\kappa+R_a-R_e)(t-t')-\kappa\tau+i(\delta+m\omega)\tau} \langle \hat\Lambda_z(t')\hat\Lambda_z(t'-\tau) \\
&= \frac{1}{(\kappa+R_a-R_e)(2\gamma+i\delta)}.
\end{aligned} \tag{S25}$$

As a result, $\langle a_d^\dagger a_d^\dagger a_d a_d\rangle / \langle a_d^\dagger a_d\rangle^2 \lesssim \kappa/\gamma \approx 10^{-3}$ under typical experimental conditions [S2]. Because of this large suppression, we neglect the term $\langle a_d^\dagger a_d^\dagger a_d a_d\rangle$ when calculating $g^{(2)}(0)$.

## GAIN OSCILLATIONS AWAY FROM THERMAL RESONANCES

As mentioned in the main text, away from the thermal resonances we generically observe strong oscillations between gain and loss. Unlike near the thermal resonances, the gain, in this case, is not phonon-assisted and instead arises from resonant transitions between Floquet quasi-energy states. Figure S2 shows the gain $G = \kappa^2/(R_e - R_a - \kappa)^2$ as a function of $A$ and $\epsilon_0$ for a drive frequency $\omega_c/\omega = 0.75$ far away from the thermal resonances.

---


[S1] M. O. Scully and S. Zubairy, *Quantum Optics* (Cambridge University Press, 1997).

[S2] Y.-Y. Liu, K. D. Petersson, J. Stehlik, J. M. Taylor, and J. R. Petta, *Photon emission from a cavity-coupled double quantum dot*, Phys. Rev. Lett. **113**, 036801 (2014).

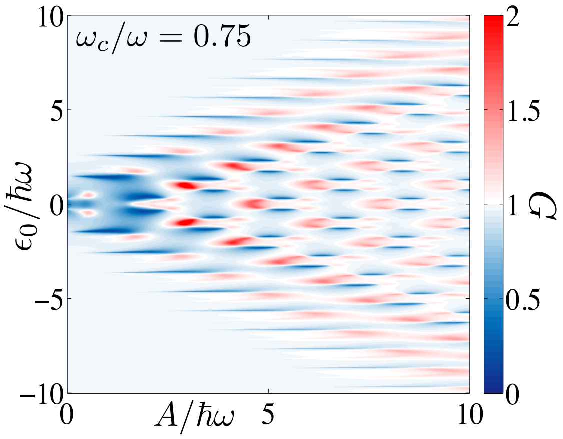


FIG. S2: (a) Normalized gain $G$ for fixed $\omega_c/\omega = 0.75$ and varying $A$ and $\epsilon_0$. We took $\omega_c/2\pi = 7.5$ GHz, $t_c = 20$ $\mu$eV, $\epsilon_0 = 0$, $g_c/2\pi = 70$ MHz, $\kappa/2\pi = 1.3$ MHz, $\eta = 5$ ns$^{-1}$, and $T = 200$ mK.
